# Supplementary material for: Comparative Study of State-of-the-Art Matrix-Product-State Methods for Lattice Models with Large Local Hilbert Spaces
Source: arXiv:2011.07412 source file (2021-09-30)
Supplement: Supplementary file 1 [file appendix.tex]

\section{Scaling Analysis in the \gls{CDW} Phase varying $\omega_0$}
\immediate\write18{head -n 1 data/holstein/L_51_N_25_t_1p0_w_0p2_g_0p6/ediff.symmps.gnu | sed -e "s/\#//g" > symmps.dat.tmp}
\pgfplotstableread[header=false,comment chars=!]{symmps.dat.tmp}{\dat}
\input{evaluate}
\pgfmathsetmacro\EminWOpIIGOpVI{\Emin}

\immediate\write18{head -n 1 data/holstein/L_51_N_25_t_1p0_w_4p0_g_10p0/ediff.symmps.gnu | sed -e "s/\#//g" > symmps.dat.tmp}
\pgfplotstableread[header=false,comment chars=!]{symmps.dat.tmp}{\dat}
\input{evaluate}
\pgfmathsetmacro\EminWIVpOGXpO{\Emin}

\begin{figure}[t!]
	\centering
	\subfloat[\label{fig:gs-energy-distance:t-1p0:w-0p2:g-0p6}]
	{
		\tikzset{external/export next=false}
		\begin{tikzpicture}
			\begin{axis}
			[
				name	    = dE,
				xmajorgrids = true,
				ymajorgrids = true,
				width	= 0.45\textwidth,
				height	= 0.25\textheight,
				ymode	= log,
				xlabel	= {$m_{\mathrm{max}}$},
				ylabel	= {$\Delta E$},
				title	= {$\omega_0/t=0.2,$ $\gamma/t=0.6$, $E_{\rm min}/t=$ \pgfmathprintnumber[fixed, precision=16]{\EminWOpIIGOpVI}},
				title style	= {font=\scriptsize},
				ticklabel style	= {font=\scriptsize},
				xlabel style	= {font=\scriptsize,yshift=0pt},
				ylabel style	= {font=\scriptsize,yshift=0pt},
			]	
				\addplot
				[
					color			= colorB,
					mark			= x,
					unbounded coords	= jump,
					thick,
				]
				table
				[
					x expr	= \thisrowno{0}/3,
					y expr	= \thisrowno{1},
				]
				{data/holstein/L_51_N_25_t_1p0_w_0p2_g_0p6/ediff.symmps.mkl}; \label{pl:m-de:symmps:w-0p2:g-0p6}
				
				\addplot
				[
					color			= colorC,
					mark			= o,
					unbounded coords	= jump,
					thick,
				]
				table
				[
					x expr	= \thisrowno{0},
					y expr	= \thisrowno{1},
				]
				{data/holstein/L_51_N_25_t_1p0_w_0p2_g_0p6/ediff.dmrg3s.nph.31.do.5}; \label{pl:m-de:lbo:w-0p2:g-0p6:n-31:d-5}
				
				\addplot
				[
					color			= colorC,
					mark			= +,
					unbounded coords	= jump,
					thick,
				]
				table
				[
					x expr	= \thisrowno{0},
					y expr	= \thisrowno{1},
				]
				{data/holstein/L_51_N_25_t_1p0_w_0p2_g_0p6/ediff.dmrg3s.nph.31.do.7}; \label{pl:m-de:lbo:w-0p2:g-0p6:n-31:d-7}
				
				\addplot
				[
					color			= colorD,
					mark			= o,
					unbounded coords	= jump,
					thick,
				]
				table
				[
					x expr	= \thisrowno{0},
					y expr	= \thisrowno{1},
				]
				{data/holstein/L_51_N_25_t_1p0_w_0p2_g_0p6/ediff.dmrg3s.nph.63.do.5}; \label{pl:m-de:lbo:w-0p2:g-0p6:n-63:d-5}
				
				\addplot
				[
					color			= colorD,
					mark			= +,
					unbounded coords	= jump,
					thick,
				]
				table
				[
					x expr	= \thisrowno{0},
					y expr	= \thisrowno{1},
				]
				{data/holstein/L_51_N_25_t_1p0_w_0p2_g_0p6/ediff.dmrg3s.nph.63.do.7}; \label{pl:m-de:lbo:w-0p2:g-0p6:n-63:d-7}
				
				\addplot
				[
					color			= colorC,
					mark			= square,
					unbounded coords	= jump,
					thick,
				]
				table
				[
					x expr	= \thisrowno{0},
					y expr	= \thisrowno{1},
				]
				{data/holstein/L_51_N_25_t_1p0_w_0p2_g_0p6/ediff.pseudo_site.nph.31}; \label{pl:m-de:ps:w-0p2:g-0p6:n-31}
				
				\addplot
				[
					color			= colorD,
					mark			= square,
					unbounded coords	= jump,
					thick,
				]
				table
				[
					x expr	= \thisrowno{0},
					y expr	= \thisrowno{1},
				]
				{data/holstein/L_51_N_25_t_1p0_w_0p2_g_0p6/ediff.pseudo_site.nph.63}; \label{pl:m-de:ps:w-0p2:g-0p6:n-63}
			\end{axis}
			\node[draw,fill=white,inner sep=1pt,below=2.5em, anchor=north] at (dE.south)
			{
				\scriptsize
				\begin{tabular}{ccc}
					\multicolumn{3}{c}{PP-2DMRG} \\
					\multicolumn{3}{c}{\ref{pl:m-de:symmps:w-0p2:g-0p6} $m_{\rm max}/3$} \\
					&& \\
					\multicolumn{3}{c}{\gls{PS-DMRG}} \\
					\multicolumn{3}{c}{\ref{pl:m-de:ps:w-0p2:g-0p6:n-31} $m_{\rm max}, n_{\rm ph}=31$} \\
					\multicolumn{3}{c}{\ref{pl:m-de:ps:w-0p2:g-0p6:n-63} $m_{\rm max}, n_{\rm ph}=63$} \\
				\end{tabular}
				
				\scriptsize
				\begin{tabular}{ccc}
					\multicolumn{3}{c}{\gls{DMRG3S+LBO}}\\
					$31$ & $63$ & $\nicefrac{n_{\rm ph}}{d_{\rm o}}$ \\
					\ref{pl:m-de:lbo:w-0p2:g-0p6:n-31:d-5} & \ref{pl:m-de:lbo:w-0p2:g-0p6:n-63:d-5} & $5$\\
					\ref{pl:m-de:lbo:w-0p2:g-0p6:n-31:d-7} & \ref{pl:m-de:lbo:w-0p2:g-0p6:n-63:d-7} & $7$
				\end{tabular}
			};
		\end{tikzpicture}
	}\\
	\subfloat[\label{fig:gs-var-energy:t-1p0:w-0p2:g-0p6}]
	{
		\tikzset{external/export next=false}
		\begin{tikzpicture}
			\begin{axis}
			[
				name	    = dE,
				xmajorgrids = true,
				ymajorgrids = true,
				width	= 0.45\textwidth,
				height	= 0.25\textheight,
				xmode	= log,
				ymode	= log,
				xlabel	= {$\operatorname{Var}[\hat H]$},
				ylabel	= {$\Delta E$},
				title	= {$\omega_0/t=0.2,$ $\gamma/t=0.6$},
				title style	= {font=\scriptsize},
				ticklabel style	= {font=\scriptsize},
				xlabel style	= {font=\scriptsize,yshift=0pt},
				ylabel style	= {font=\scriptsize,yshift=0pt},
			]	
				\addplot
				[
					color			= colorB,
					mark			= x,
					unbounded coords	= jump,
					thick,
				]
				table
				[
					x expr	= \thisrowno{2},
					y expr	= \thisrowno{1},
				]
				{data/holstein/L_51_N_25_t_1p0_w_0p2_g_0p6/ediff.symmps.mkl}; \label{pl:var-de:symmps:w-0p2:g-0p6}
				
				\addplot
				[
					color			= colorC,
					mark			= o,
					unbounded coords	= jump,
					thick,
				]
				table
				[
					x expr	= \thisrowno{2},
					y expr	= \thisrowno{1},
				]
				{data/holstein/L_51_N_25_t_1p0_w_0p2_g_0p6/ediff.dmrg3s.nph.31.do.5}; \label{pl:var-de:lbo:w-0p2:g-0p6:n-31:d-5}
				
				\addplot
				[
					color			= colorC,
					mark			= +,
					unbounded coords	= jump,
					thick,
				]
				table
				[
					x expr	= \thisrowno{2},
					y expr	= \thisrowno{1},
				]
				{data/holstein/L_51_N_25_t_1p0_w_0p2_g_0p6/ediff.dmrg3s.nph.31.do.7}; \label{pl:var-de:lbo:w-0p2:g-0p6:n-31:d-7}
				
				\addplot
				[
					color			= colorD,
					mark			= o,
					unbounded coords	= jump,
					thick,
				]
				table
				[
					x expr	= \thisrowno{2},
					y expr	= \thisrowno{1},
				]
				{data/holstein/L_51_N_25_t_1p0_w_0p2_g_0p6/ediff.dmrg3s.nph.63.do.5}; \label{pl:var-de:lbo:w-0p2:g-0p6:n-63:d-5}
				
				\addplot
				[
					color			= colorD,
					mark			= +,
					unbounded coords	= jump,
					thick,
				]
				table
				[
					x expr	= \thisrowno{2},
					y expr	= \thisrowno{1},
				]
				{data/holstein/L_51_N_25_t_1p0_w_0p2_g_0p6/ediff.dmrg3s.nph.63.do.7}; \label{pl:var-de:lbo:w-0p2:g-0p6:n-63:d-7}
			\end{axis}
			\node[draw,fill=white,inner sep=1pt,above left=-0.25em, anchor=north west] at (dE.north west) 
			{
				\scriptsize
				\begin{tabular}{ccc}
					\multicolumn{3}{c}{PP-2DMRG} \\
					\multicolumn{3}{c}{\ref{pl:var-de:symmps:w-0p2:g-0p6} $m_{\rm max}/3$} \\
					&& \\
					\multicolumn{3}{c}{\gls{DMRG3S+LBO}}\\
					$31$ & $63$ & $\nicefrac{n_{\rm ph}}{d_{\rm o}}$ \\
					\ref{pl:var-de:lbo:w-0p2:g-0p6:n-31:d-5} & \ref{pl:var-de:lbo:w-0p2:g-0p6:n-63:d-5} & $5$\\
					\ref{pl:var-de:lbo:w-0p2:g-0p6:n-31:d-7} & \ref{pl:var-de:lbo:w-0p2:g-0p6:n-63:d-7} & $7$
				\end{tabular}
			};
		\end{tikzpicture}
	}
	\caption
	{
		\label{fig:t-1p0:w-0p2:g-0p6}
		Relative distance to minimally found ground state energies \protect\subref{fig:gs-energy-distance:t-1p0:w-0p2:g-0p6} and its scaling w.r.t.~the variance \protect\subref{fig:gs-var-energy:t-1p0:w-0p2:g-0p6} using \gls{PS-DMRG} ($\Delta E$ only), \gls{PP-2DMRG} and \gls{DMRG3S+LBO} varying maximal bond dimensions (both), number of phonons and optimal modes (DMRG3S) for parameter set \eqref{eq:comp-pp-with-lbo:4}.
	}
\end{figure}
\begin{figure}[t!]
	\centering
	\subfloat[\label{fig:gs-energy-distance:t-1p0:w-4p0:g-10p0}]
	{
		\tikzset{external/export next=false}
		\begin{tikzpicture}
			\begin{axis}
			[
				name	    = dE,
				xmajorgrids = true,
				ymajorgrids = true,
				width	= 0.45\textwidth,
				height	= 0.25\textheight,
				ymode	= log,
				xlabel	= {$m_{\mathrm{max}}$},
				ylabel	= {$\Delta E$},
				title	= {$\omega_0/t=4.0,$ $\gamma/t=10.0$, $E_{\rm min}/t=$ \pgfmathprintnumber[fixed, precision=16]{\EminWIVpOGXpO}},
				title style	= {font=\scriptsize},
				ticklabel style	= {font=\scriptsize},
				xlabel style	= {font=\scriptsize,yshift=0pt},
				ylabel style	= {font=\scriptsize,yshift=0pt},
			]	
				\addplot
				[
					color			= colorB,
					mark			= x,
					unbounded coords	= jump,
					thick,
				]
				table
				[
					x expr	= \thisrowno{0}/2,
					y expr	= \thisrowno{1},
				]
				{data/holstein/L_51_N_25_t_1p0_w_4p0_g_10p0/ediff.symmps.mkl}; \label{pl:m-de:symmps:w-4p0:g-10p0}
				
				\addplot
				[
					color			= colorC,
					mark			= o,
					unbounded coords	= jump,
					thick,
				]
				table
				[
					x expr	= \thisrowno{0},
					y expr	= \thisrowno{1},
				]
				{data/holstein/L_51_N_25_t_1p0_w_4p0_g_10p0/ediff.dmrg3s.nph.63.do.5}; \label{pl:m-de:lbo:w-4p0:g-10p0:n-63:d-5}
				
				\addplot
				[
					color			= colorC,
					mark			= +,
					unbounded coords	= jump,
					thick,
				]
				table
				[
					x expr	= \thisrowno{0},
					y expr	= \thisrowno{1},
				]
				{data/holstein/L_51_N_25_t_1p0_w_4p0_g_10p0/ediff.dmrg3s.nph.63.do.7}; \label{pl:m-de:lbo:w-4p0:g-10p0:n-63:d-7}
				
				\addplot
				[
					color			= colorD,
					mark			= o,
					unbounded coords	= jump,
					thick,
				]
				table
				[
					x expr	= \thisrowno{0},
					y expr	= \thisrowno{1},
				]
				{data/holstein/L_51_N_25_t_1p0_w_4p0_g_10p0/ediff.dmrg3s.nph.127.do.5}; \label{pl:m-de:lbo:w-4p0:g-10p0:n-127:d-5}
				
				\addplot
				[
					color			= colorD,
					mark			= +,
					unbounded coords	= jump,
					thick,
				]
				table
				[
					x expr	= \thisrowno{0},
					y expr	= \thisrowno{1},
				]
				{data/holstein/L_51_N_25_t_1p0_w_4p0_g_10p0/ediff.dmrg3s.nph.127.do.7}; \label{pl:m-de:lbo:w-4p0:g-10p0:n-127:d-7}
				
				\addplot
				[
					color			= colorC,
					mark			= square,
					unbounded coords	= jump,
					thick,
				]
				table
				[
					x expr	= \thisrowno{0}/2,
					y expr	= \thisrowno{1},
				]
				{data/holstein/L_51_N_25_t_1p0_w_4p0_g_10p0/ediff.pseudo_site.nph.63}; \label{pl:m-de:ps:w-4p0:g-10p0:n-63}
				
				\addplot
				[
					color			= colorD,
					mark			= square,
					unbounded coords	= jump,
					thick,
				]
				table
				[
					x expr	= \thisrowno{0}/2,
					y expr	= \thisrowno{1},
				]
				{data/holstein/L_51_N_25_t_1p0_w_4p0_g_10p0/ediff.pseudo_site.nph.127}; \label{pl:m-de:ps:w-4p0:g-10p0:n-127}
			\end{axis}
			\node[draw,fill=white,inner sep=1pt,below=2.5em, anchor=north] at (dE.south)
			{
				\scriptsize
				\begin{tabular}{ccc}
					\multicolumn{3}{c}{PP-2DMRG} \\
					\multicolumn{3}{c}{\ref{pl:m-de:symmps:w-4p0:g-10p0} $m_{\rm max}/2$} \\
					&& \\
					\multicolumn{3}{c}{\gls{PS-DMRG}} \\
					\multicolumn{3}{c}{\ref{pl:m-de:ps:w-4p0:g-10p0:n-63} $m_{\rm max}/2, n_{\rm ph}=\phantom{1}63$} \\
					\multicolumn{3}{c}{\ref{pl:m-de:ps:w-4p0:g-10p0:n-127} $m_{\rm max}/2, n_{\rm ph}=127$}
				\end{tabular}
				
				\scriptsize
				\begin{tabular}{ccc}
					\multicolumn{3}{c}{\gls{DMRG3S+LBO}}\\
					\centeredSplittedTableHeader{$n_{\rm ph}$}{$d_{\rm o}$} & $63$ & $127$ \\
					$5$ & \ref{pl:m-de:lbo:w-4p0:g-10p0:n-63:d-5} & \ref{pl:m-de:lbo:w-4p0:g-10p0:n-127:d-5}\\
					$7$ & \ref{pl:m-de:lbo:w-4p0:g-10p0:n-63:d-7} & \ref{pl:m-de:lbo:w-4p0:g-10p0:n-127:d-7}
				\end{tabular}
			};
		\end{tikzpicture}
	}\\
	\subfloat[\label{fig:gs-var-energy:t-1p0:w-4p0:g-10p0}]
	{
		\tikzset{external/export next=false}
		\begin{tikzpicture}
			\begin{axis}
			[
				name	    = dE,
				xmajorgrids = true,
				ymajorgrids = true,
				width	= 0.45\textwidth,
				height	= 0.25\textheight,
				xmode	= log,
				ymode	= log,
				xlabel	= {$\operatorname{Var}[\hat H]$},
				ylabel	= {$\Delta E$},
				title	= {$\omega_0/t=4.0,$ $\gamma/t=10.0$},
				title style	= {font=\scriptsize},
				ticklabel style	= {font=\scriptsize},
				xlabel style	= {font=\scriptsize,yshift=0pt},
				ylabel style	= {font=\scriptsize,yshift=0pt},
			]	
				\addplot
				[
					color			= colorB,
					mark			= x,
					unbounded coords	= jump,
					thick,
				]
				table
				[
					x expr	= \thisrowno{2},
					y expr	= \thisrowno{1},
				]
				{data/holstein/L_51_N_25_t_1p0_w_4p0_g_10p0/ediff.symmps.mkl}; \label{pl:var-de:symmps:w-4p0:g-10p0}
				
				\addplot
				[
					color			= colorC,
					mark			= o,
					unbounded coords	= jump,
					thick,
				]
				table
				[
					x expr	= \thisrowno{2},
					y expr	= \thisrowno{1},
				]
				{data/holstein/L_51_N_25_t_1p0_w_4p0_g_10p0/ediff.dmrg3s.nph.63.do.5}; \label{pl:var-de:lbo:w-4p0:g-10p0:n-63:d-5}
				
				\addplot
				[
					color			= colorC,
					mark			= +,
					unbounded coords	= jump,
					thick,
				]
				table
				[
					x expr	= \thisrowno{2},
					y expr	= \thisrowno{1},
				]
				{data/holstein/L_51_N_25_t_1p0_w_4p0_g_10p0/ediff.dmrg3s.nph.63.do.7}; \label{pl:var-de:lbo:w-4p0:g-10p0:n-63:d-7}
				
				\addplot
				[
					color			= colorD,
					mark			= o,
					unbounded coords	= jump,
					thick,
				]
				table
				[
					x expr	= \thisrowno{2},
					y expr	= \thisrowno{1},
				]
				{data/holstein/L_51_N_25_t_1p0_w_4p0_g_10p0/ediff.dmrg3s.nph.127.do.5}; \label{pl:var-de:lbo:w-4p0:g-10p0:n-127:d-5}
				
				\addplot
				[
					color			= colorD,
					mark			= +,
					unbounded coords	= jump,
					thick,
				]
				table
				[
					x expr	= \thisrowno{2},
					y expr	= \thisrowno{1},
				]
				{data/holstein/L_51_N_25_t_1p0_w_4p0_g_10p0/ediff.dmrg3s.nph.127.do.7}; \label{pl:var-de:lbo:w-4p0:g-10p0:n-127:d-7}
			\end{axis}
% 			\node[draw,fill=white,inner sep=1pt,above left=-0.25em, anchor=north west] at (dE.north west) 
% 			{
% 				\scriptsize
% 				\begin{tabular}{ccc}
% 					\multicolumn{3}{c}{\gls{PP-2DMRG} \ref{pl:var-de:symmps:w-4p0:g-10p0}} \\
% 					&& \\
% 					\multicolumn{3}{c}{\gls{DMRG3S+LBO}}\\
% 					\centeredSplittedTableHeader{$n_{\rm ph}$}{$d_{\rm o}$} & $63$ & $127$ \\
% 					$5$ & \ref{pl:m-de:lbo:w-4p0:g-10p0:n-63:d-5} & \ref{pl:m-de:lbo:w-4p0:g-10p0:n-127:d-5}\\
% 					$7$ & \ref{pl:m-de:lbo:w-4p0:g-10p0:n-63:d-7} & \ref{pl:m-de:lbo:w-4p0:g-10p0:n-127:d-7}
% 				\end{tabular}
% 			};
		\end{tikzpicture}
	}
	\caption
	{
		\label{fig:t-1p0:w-4p0:g-10p0}
		Relative distance to minimally found ground state energies \protect\subref{fig:gs-energy-distance:t-1p0:w-4p0:g-10p0} and its scaling w.r.t.~the variance \protect\subref{fig:gs-var-energy:t-1p0:w-4p0:g-10p0} using \gls{PS-DMRG} ($\Delta E$ only), \gls{PP-2DMRG} and \gls{DMRG3S+LBO} varying maximal bond dimensions (both), number of phonons and optimal modes (DMRG3S) for parameter set \eqref{eq:comp-pp-with-lbo:5}.
	}
\end{figure}
\section{Finite Size Scaling in the \gls{LL} and \gls{CDW} phase}

\def\Ls{51, 101, 151, 201, 301}
\def\dws{1em04, 1em06, 1em08, 1em10}
\def\dw{1em08}

\def\t{1p0}
\def\w{1p0}
\def\g{0p5}
\def\blas{mkl}
\def\m{2000}
\def\nph{63}
\def\nphlbo{31}
\def\xmin{1e-10}%
\def\xmax{2e-4}%
\def\xminMain{9e-4}%
\def\ocgname{p}%
\def\dataroot{data/holstein/symmps_with_bath_sites/}
\edef\datadir{\dataroot/t_\noexpand\t_w_\noexpand\w_g_\noexpand\g/finite_size_scaling/L_\noexpand\L_N_\noexpand\N/\noexpand\blas/m_\noexpand\m_d_\noexpand\d_nph_\noexpand\nph}
\edef\dstdir{\dataroot/t_\noexpand\t_w_\noexpand\w_g_\noexpand\g/finite_size_scaling}
\setboolean{removeData}{true}%
\setboolean{rebuildData}{true}%
\def\captionContent{%
	\label{fig:ppdmrg:finite-size-scaling:t-\t_w-\w_g-\g:site_25}
	Finite size scaling for the groundstate energy of the Holstein model.
	The model is evaluated for parameters $\omega/t=\protect\ReplaceStr{\w}$, $\gamma/t=\protect\ReplaceStr{\g}$ at nearly half filling where we set $N_{\rm el}=\frac{L-1}{2}$.
	The inset shows the total CPU time for the groundstate search as a function of the number of lattice sites $L$.
}%
\setboolean{removeData}{true}%
\def\dataroot{data/holstein/symmps_with_bath_sites/}%
\edef\datadir{\dataroot/t_\noexpand\t_w_\noexpand\w_g_\noexpand\g/finite_size_scaling/L_\noexpand\L_N_\noexpand\N/\noexpand\blas/m_\noexpand\m_d_\noexpand\d_nph_\noexpand\nph}%
\edef\dstdir{\dataroot/t_\noexpand\t_w_\noexpand\w_g_\noexpand\g/finite_size_scaling}%
\ifthenelse{\boolean{rebuildData}}%
{%
	%		\immediate\write18{bash -c "export t=\t; export w=\w; export g=\g; export nph=\nph; export dw=\dw; python3 data/holstein/build_finite_size_scaling_datatable.py --t-hop \string\${t/\string\p/\string\.} --omega \string\${w/\string\p/\string\.} --gamma \string\${g/\string\p/\string\.} --n-phonons \string\${nph/\string\p/\string\.} --disc-wt \string\${dw/\string\p/\string\.} --root-dir data/holstein --out-file data/holstein/finite_size_scaling/t_\t_w_\w_g_\g" >&2}%
}{}%
\setboolean{rebuildCurrentBlock}{false}%
\setboolean{buildCurrentBlockInline}{true}%
\ifthenelse{\boolean{rebuildCurrentBlock}}%
{%
	\setboolean{removeData}{true}%
}%
{%
	\ifthenelse{\boolean{buildCurrentBlockInline}}%
	{%
		\setboolean{removeData}{true}%
	}{}%
}%
\ifthenelse{\boolean{removeData}}%
{%
	\immediate\write18{rm -f \dstdir/scaling.dat}%
}{}%
\foreach \L in \Ls%
{%
	\immediate\write18{echo "L: \L" 1>&2}%
	\pgfmathsetmacro{\N}{int(\L/2)}%
%	N=\N%
%
	\def\d{1em04}%
	\immediate\write18{echo "dw E0 convergence discweight" > \datadir/../gs_energies.dat}%%
%	\IfFileExists{\datadir/../gs_fit.dat}{\immediate\write18{rm -f \datadir/../gs_fit.dat}}{}%
%
	\foreach \d in \dws%
	{%
		\ifthenelse{\boolean{rebuildCurrentBlock}}%
		{%
			\IfFileExists{\datadir/log/sym-groundstate-search.output}%
			{%
				\setboolean{rebuildData}{true}%
			}%
			{%
				\setboolean{rebuildData}{false}%		
			}%
		}%
		{%
			\ifthenelse{\boolean{buildCurrentBlockInline}}%
			{%
				\IfFileExists{\datadir/log/sym-groundstate-search.output}%
				{%
					\setboolean{rebuildData}{true}%
				}%
				{%
					\setboolean{rebuildData}{false}%
				}%
			}%
			{%
				\setboolean{rebuildData}{false}%
			}%
		}%
		\ifthenelse{\boolean{rebuildData}}%
		{%
			\immediate\write18{rm -f \datadir/../.NoValidResultsDetected.tmp}%
			\immediate\write18%
			{%
				if [ \string$(grep '\string^energy' \datadir/log/sym-groundstate-search.output | wc -l) = 0 ]; then touch  \datadir/../.NoValidResultsDetected.tmp; fi
			}%
			\IfFileExists{\datadir/.not_converged}%
			{%
				\immediate\write18{touch  \datadir/../.NoValidResultsDetected.tmp}%
			}{}%
			\IfFileExists{\datadir/../.NoValidResultsDetected.tmp}%
			{%
				\immediate\write18{rm -f \datadir/../.NoValidResultsDetected.tmp}%
			}%
			{%	
%				\immediate\write18%
%				{%
%					echo \d	\
%					\string$(grep -B3 'stage \stage c' \datadir/log/sym-groundstate-search.output | tail -n3 | head -n1 | tr -d , | awk '{print \string$2,\string"\string\t\string",\string$5}') \
%					\string$(grep -B\string$((\L+6)) 'stage \stage c' \datadir/log/sym-groundstate-search.output | tail -n \string$((\L+6)) | sed "s/e-gain /e-gain:/" | awk "{print \string\$12}" | LC_NUMERIC=en_US.UTF-8 sort -g | tail -n1 )	\
%					>>  \datadir/../gs_energies.dat
%				}%
				\immediate\write18%
				{%
					echo \d	\
					\string$(grep '\string^energy' \datadir/log/sym-groundstate-search.output | tail -n1 | tr -d , | awk '{print \string$2,\string"\string\t\string",\string$5}') \
					\string$(grep -B\string$((\L+4)) '\string^energy' \datadir/log/sym-groundstate-search.output | tail -n \string$((\L+4)) | sed "s/e-gain /e-gain:/" | awk "{print \string\$12}" | LC_NUMERIC=en_US.UTF-8 sort -g | tail -n1 )	\
					>>  \datadir/../gs_energies.dat
				}%
			}%
		}{}%
	}%
	\IfFileExists{\datadir/../gs_energies.dat}%
	{
		\immediate\write18%
		{if [ \string$(cat \datadir/../gs_energies.dat | wc -l) = 1 ]; then touch  \datadir/../.NoValidResultsDetected.tmp; fi}%
	}%
	{
		\immediate\write18{touch  \datadir/../.NoValidResultsDetected.tmp}%	
	}%
	\IfFileExists{\datadir/../.NoValidResultsDetected.tmp}%
	{}%
	{%
		\IfFileExists{\datadir/log/sym-groundstate-search.output}%
		{%
			\ifthenelse{\boolean{rebuildCurrentBlock}}%
			{%
				\tikzset{external/remake next=true}%
				\IfFileExists{\datadir/../gs_fit.dat}{\immediate\write18{rm -f \datadir/../gs_fit.dat}}{}%
			}%
			{%
				\ifthenelse{\boolean{buildCurrentBlockInline}}%
				{%
					\tikzset{external/export next=false}%
					\IfFileExists{\datadir/../gs_fit.dat}{\immediate\write18{rm -f \datadir/../gs_fit.dat}}{}%
				}{}%
			}%
			\begin{tikzpicture}%
				\begin{axis}
				[
					opacity	= 0,
					width	=	0.85\textwidth,
					height	=	0.25\textheight,
					xmode	=	log,
					xlabel	=	{\small Discarded weight},
					ylabel	=	{$\nicefrac{E_0}{L}$},
					legend pos	=	north west,
					legend style=
					{
						font=\tiny,
					},
				]
				\addplot
				[
					color=blue,
					thick,
					only marks,
					mark=x,
					unbounded coords=jump,
					error bars/.cd, 
					y dir=both,
					y explicit,
				] 
					table
					[
						x expr = \thisrowno{3},
						y expr = \thisrowno{1}/(\L),
						y error expr = 2.0*sqrt(\thisrowno{3}/\L), 
					]
					{\datadir/../gs_energies.dat};
				\addlegendentry{DMRG results};
				
				\makeatletter
					\addplot
					[
						no markers, 
						color=blue,
						thick,
					] 
						gnuplot 
						[
							raw gnuplot
						] 
						{
							set fit quiet;
							set fit logfile '/dev/null';
							set print "\datadir/../gs_fit.dat" append;
							set fit errorvariables;
							f(x) = a+abs(b)*x;
							fit f(x) '\datadir/../gs_energies.dat' u ($4):($2) via a,b;
							fit f(x) '\datadir/../gs_energies.dat' u ($4):($2):(2.0*sqrt($4)) yerrors via a,b;
							print \L,\N,a,a_err,b,b_err;
						};
				\makeatother
				
				\IfFileExists{\datadir/../gs_fit.dat}%
				{
					\immediate\write18%
					{if [ \string$(cat \datadir/../gs_fit.dat | wc -l) = 0 ]; then touch  \datadir/../.NoValidFit.tmp; fi}%
				}%
				{
					\immediate\write18{touch  \datadir/../.NoValidResultsDetected.tmp}%	
				}%
				
				\IfFileExists{\datadir/../.NoValidFit.tmp}%
				{
					\immediate\write18{rm -f \datadir/../.NoValidFit.tmp}%	
					\immediate\write18{rm -f \datadir/../.NoValidResultsDetected.tmp}%	
				}
				{
					\pgfplotstableread[header=false]{\datadir/../gs_fit.dat}{\DataUZero}
					\pgfplotstablegetelem{0}{2}\of\DataUZero 
					\pgfmathsetmacro{\Ea}{\pgfplotsretval}
					\pgfplotstablegetelem{0}{3}\of\DataUZero 
					\edef\Eaerr{\pgfplotsretval}
					\pgfplotstablegetelem{0}{4}\of\DataUZero 
					\pgfmathsetmacro{\Eb}{\pgfplotsretval}
					
					\addplot
					[
						domain	=	\xmin:\xmax,
						color=blue,
						dashed,
					]
						{linearFct(\Eb, \Ea)/\L};
					\pgfmathparse{\Ea/\L}
					\edef\E{\pgfmathresult}
					\addlegendentry{fit to $E_0/L=\pgfmathprintnumber[std,precision=4]{\E} \pm \pgfmathprintnumber[sci,precision=2]{\Eaerr}$};
				}
				\end{axis}
			\end{tikzpicture}%
		}{}%
		\IfFileExists{\datadir/../gs_fit.dat}%
		{%
			\immediate\write18%
			{%
				grep -v "inf.0" \datadir/../gs_fit.dat | grep -v "NaN" >> \dstdir/scaling.dat
			}%
		}{}%
	}%
}%
\ifthenelse{\boolean{rebuildCurrentBlock}}%
{%
	\IfFileExists{\datadir/log/sym-groundstate-search.output}%
	{%
		\setboolean{rebuildData}{true}%
	}%
	{%
		\setboolean{rebuildData}{false}%		
	}%
}%
{%
	\ifthenelse{\boolean{buildCurrentBlockInline}}%
	{%
		\setboolean{rebuildData}{true}%
	}%
	{%
		\setboolean{rebuildData}{false}%
	}%
}%
\vspace{-0.24\textheight}%
\ifthenelse{\boolean{removeData}}%
{%
	\immediate\write18{rm -f data/holstein/finite_size_scaling/t_\t_w_\w_g_\g*gs_energy_fit}%
	\immediate\write18{rm -f \dstdir/scaling_output.dat}%
	\setboolean{rebuildData}{true}%
}{}%
\setboolean{rebuildCurrentBlock}{false}%
\setboolean{buildCurrentBlockInline}{true}%
\begin{figure}[!t]
	\centering
	\input{the_actual_finite_size_scaling_plot}%
	\caption
	{
		\captionContent
	}
\end{figure}%
\setboolean{removeData}{false}%

\def\Ls{51, 101, 151, 201, 251, 301, 401, 501, 601, 701, 801, 901, 1001}
\def\dws{1em04, 1em06, 1em08, 1em10}
\def\dw{1em08}

\def\t{1p0}
\def\w{1p0}
\def\g{1p5}
\def\blas{mkl}
\def\m{2000}
\def\nph{63}
\def\nphlbo{31}
\def\xmin{1e-10}%
\def\xmax{2e-4}%
\def\xminMain{9e-4}%
\def\ocgname{p}%
\def\dataroot{data/holstein/symmps_with_bath_sites/}
\edef\datadir{\dataroot/t_\noexpand\t_w_\noexpand\w_g_\noexpand\g/finite_size_scaling/L_\noexpand\L_N_\noexpand\N/\noexpand\blas/m_\noexpand\m_d_\noexpand\d_nph_\noexpand\nph}
\edef\dstdir{\dataroot/t_\noexpand\t_w_\noexpand\w_g_\noexpand\g/finite_size_scaling}
\setboolean{removeData}{true}%
\setboolean{rebuildData}{true}%
\def\captionContent{%
	\label{fig:ppdmrg:finite-size-scaling:t-\t_w-\w_g-\g:site_25}
	Finite size scaling for the groundstate energy of the Holstein model.
	The model is evaluated for parameters $\omega/t=\protect\ReplaceStr{\w}$, $\gamma/t=\protect\ReplaceStr{\g}$ at nearly half filling where we set $N_{\rm el}=\frac{L-1}{2}$.
	The inset shows the total CPU time for the groundstate search as a function of the number of lattice sites $L$.
}%

\def\Ls{51, 101, 151, 201}
\def\dws{1em04, 1em06, 1em08, 1em10}
\def\dw{1em08}

\def\dw{1em08}
\def\t{1p0}
\def\w{1p0}
\def\g{2p0}
\def\blas{mkl}
\def\m{2000}
\def\nph{63}
\def\nphlbo{31}
\def\xmin{1e-10}%
\def\xmax{2e-4}%
\def\xminMain{9e-4}%
\def\ocgname{ppp}%
\def\dataroot{data/holstein/symmps_with_bath_sites/}
\edef\datadir{\dataroot/t_\noexpand\t_w_\noexpand\w_g_\noexpand\g/finite_size_scaling/L_\noexpand\L_N_\noexpand\N/\noexpand\blas/m_\noexpand\m_d_\noexpand\d_nph_\noexpand\nph}
\edef\dstdir{\dataroot/t_\noexpand\t_w_\noexpand\w_g_\noexpand\g/finite_size_scaling}
\setboolean{removeData}{true}%
\setboolean{rebuildData}{true}%
\def\captionContent{%
	\label{fig:ppdmrg:finite-size-scaling:t-\t_w-\w_g-\g:site_25}
	Finite size scaling for the groundstate energy of the Holstein model.
	The model is evaluated for parameters $\omega/t=\protect\ReplaceStr{\w}$, $\gamma/t=\protect\ReplaceStr{\g}$ at nearly half filling where we set $N_{\rm el}=\frac{L-1}{2}$.
	The inset shows the total CPU time for the groundstate search as a function of the number of lattice sites $L$.
}%

\def\Ls{51, 101, 151, 201, 301}
\def\dw{1em10}
\def\t{1p0}
\def\w{1p0}
\def\g{0p5}
\def\blas{mkl}
\def\m{2000}
\def\nph{63}
\def\nphlbo{31}
\def\xmin{301}%
\def\xmax{51}%
\def\legendPosition{(0.03,0.03)}%
\setboolean{rebuildCurrentBlock}{false}
\setboolean{buildCurrentBlockInline}{true}
\begin{figure}[!t]
	\centering
	\ifthenelse{\boolean{rebuildCurrentBlock}}%
	{%
		\setboolean{removeData}{true}%
		\setboolean{rebuildData}{true}%
		\tikzset{external/remake next=true}%
	}%
	{%
		\ifthenelse{\boolean{buildCurrentBlockInline}}%
		{%
			\setboolean{removeData}{true}%
			\setboolean{rebuildData}{true}%
			\tikzset{external/export next=false}%
		}{}%
	}%
	\ifthenelse{\boolean{rebuildData}}%
	{%
%		\immediate\write18{bash -c "export t=\t; export w=\w; export g=\g; export nph=\nph; export dw=\dw; python3 data/holstein/build_finite_size_scaling_datatable.py --t-hop \string\${t/\string\p/\string\.} --omega \string\${w/\string\p/\string\.} --gamma \string\${g/\string\p/\string\.} --n-phonons \string\${nph/\string\p/\string\.} --disc-wt \string\${dw/\string\p/\string\.} --root-dir data/holstein --out-file data/holstein/finite_size_scaling/t_\t_w_\w_g_\g" >&2}%
	}{}%
	\ifthenelse{\boolean{removeData}}%
	{%
		\immediate\write18{bash -c "rm -f data/holstein/finite_size_scaling/t_\t_w_\w_g_\g.*order_parameter_fit"}%
	}{}%
	\tikzsetnextfilename{PPDMRG-finite-size-scaling-order_parameter_t_\t-w_\w-g_\g}
	\begin{tikzpicture}
		\begin{axis}
		[
			width	= 0.95\textwidth,
			height	= 0.3\textheight,
			xmin	= 0,
			xmax	= 0.02,
			xlabel	= {$1/L$},
			ylabel	= {$x_{\rm ph}(L)$},
			legend style	= {font=\scriptsize, at={\legendPosition}, anchor=south west},
			legend columns	= 1,
		]
			
			\addplot
			[
				color	= colorC,
				mark	= x,
				only marks,
				thick,
				restrict expr to domain	= {1/x}{\xmax:\xmin},
			]
			table
			[
				x expr	= 1/\thisrowno{0},
				y expr	= \thisrowno{6},
			]
			{data/holstein/finite_size_scaling/t_\t_w_\w_g_\g.symmps.\dw.\blas};
			\addlegendentry{\gls{PP-2DMRG}}
			
			\ifthenelse{\boolean{rebuildData}}%
			{%
				\makeatletter
					\addplot
					[
						no markers, 
						color=blue,
						thick,
						forget plot,
					] %					
						gnuplot 
						[
							raw gnuplot
						] 
						{
							set fit quiet;
							set fit logfile '/dev/null';
							set print "data/holstein/finite_size_scaling/t_\t_w_\w_g_\g.symmps.\dw.\blas_order_parameter_fit" append;
							set fit errorvariables;
							f(x) = a+b*x+c*x*x;
							fit [1.0/\xmin:1.0/\xmax]f(x) 'data/holstein/finite_size_scaling/t_\t_w_\w_g_\g.symmps.\dw.\blas' u (1.0/$1):7 via a,b,c;
							print a,a_err,b,b_err,c,c_err;
						};
				\makeatother
			}{}%
			\pgfplotstableread[header=false]{data/holstein/finite_size_scaling/t_\t_w_\w_g_\g.symmps.\dw.\blas_order_parameter_fit}{\Data}
			\pgfplotstablegetelem{0}{0}\of\Data 
			\xdef\ppEapp{\pgfplotsretval}
			\pgfplotstablegetelem{0}{1}\of\Data 
			\xdef\ppEaerrpp{\pgfplotsretval}
			\pgfplotstablegetelem{0}{2}\of\Data 
			\xdef\ppEbpp{\pgfplotsretval}
			\pgfplotstablegetelem{0}{3}\of\Data 
			\xdef\ppEberrpp{\pgfplotsretval}
			\pgfplotstablegetelem{0}{4}\of\Data 
			\xdef\ppEcpp{\pgfplotsretval}
			\pgfplotstablegetelem{0}{5}\of\Data 

			\addplot
			[
				forget plot,
				mark	= none,
				color	= colorC,
				thick,
				domain	= 0:0.02,
				samples	= 100,
			]
			{quadFct(\ppEcpp,\ppEbpp,\ppEapp)};
			\addplot
			[
				color	= colorA,
				mark	= o,
				only marks,
				thick,
			]
			table
			[
				skip rows between index={0}{2},
				x expr	= 1/\thisrowno{0},
				y expr	= \thisrowno{3},
			]
			{data/holstein/finite_size_scaling/t_\t_w_\w_g_\g.ps};
			\addlegendentry{\gls{PS-DMRG}}
			\ifthenelse{\boolean{rebuildData}}%
			{%
				\makeatletter
				\addplot
				[
				no markers, 
				color=blue,
				thick,
				forget plot,
				] %					
				gnuplot 
				[
				raw gnuplot
				] 
				{
					set fit quiet;
					set fit logfile '/dev/null';
					set print "data/holstein/finite_size_scaling/t_\t_w_\w_g_\g.ps_order_parameter_fit" append;
					set fit errorvariables;
					f(x) = a+b*x+c*x*x;
					fit [1.0/\xmin:1.0/\xmax]f(x) 'data/holstein/finite_size_scaling/t_\t_w_\w_g_\g.ps' u (1.0/$1):($4) via a,b,c;
					print a,a_err,b,b_err,c,c_err;
				};
				\makeatother
			}{}%
			%		%			
			\pgfplotstableread[header=false]{data/holstein/finite_size_scaling/t_\t_w_\w_g_\g.ps_order_parameter_fit}{\Data}
			\pgfplotstablegetelem{0}{0}\of\Data 
			\xdef\ppEaps{\pgfplotsretval}
			\pgfplotstablegetelem{0}{1}\of\Data 
			\xdef\ppEaerrps{\pgfplotsretval}
			\pgfplotstablegetelem{0}{2}\of\Data 
			\xdef\ppEbps{\pgfplotsretval}
			\pgfplotstablegetelem{0}{3}\of\Data 
			\xdef\ppEberrps{\pgfplotsretval}
			\pgfplotstablegetelem{0}{4}\of\Data 
			\xdef\ppEcps{\pgfplotsretval}
			\pgfplotstablegetelem{0}{5}\of\Data

			\addplot
			[
				forget plot,
				mark	= none,
				color	= colorA,
				thick,
				domain	= 0:0.02,
				samples	= 100,
			]
			{quadFct(\ppEcps,\ppEbps,\ppEaps)};
			
			\addplot
			[
				color	= colorB,
				mark	= square,
				only marks,
				thick,
			]
			table
			[
				x expr	= 1/\thisrowno{0},
				y expr	= \thisrowno{6},
			]
			{data/holstein/finite_size_scaling/t_\t_w_\w_g_\g.dmrg3s};
			\addlegendentry{\gls{DMRG3S+LBO}}

			\ifthenelse{\boolean{rebuildData}}%
			{%
				\makeatletter
					\addplot
					[
						no markers, 
						color=blue,
						thick,
						forget plot,
					] %					
						gnuplot 
						[
							raw gnuplot
						] 
						{
							set fit quiet;
							set fit logfile '/dev/null';
							set print "data/holstein/finite_size_scaling/t_\t_w_\w_g_\g.dmrg3s_order_parameter_fit" append;
							set fit errorvariables;
							f(x) = a+b*x+c*x*x;
							fit [1.0/\xmin:1.0/\xmax]f(x) 'data/holstein/finite_size_scaling/t_\t_w_\w_g_\g.dmrg3s' u (1.0/$1):($7) via a,b,c;
							print a,a_err,b,b_err,c,c_err;
						};
				\makeatother
			}{}%
			%		%			
			\pgfplotstableread[header=false]{data/holstein/finite_size_scaling/t_\t_w_\w_g_\g.dmrg3s_order_parameter_fit}{\Data}
			\pgfplotstablegetelem{0}{0}\of\Data 
			\xdef\ppEalbo{\pgfplotsretval}
			\pgfplotstablegetelem{0}{1}\of\Data 
			\xdef\ppEaerrlbo{\pgfplotsretval}
			\pgfplotstablegetelem{0}{2}\of\Data 
			\xdef\ppEblbo{\pgfplotsretval}
			\pgfplotstablegetelem{0}{3}\of\Data 
			\xdef\ppEberrlbo{\pgfplotsretval}
			\pgfplotstablegetelem{0}{4}\of\Data 
			\xdef\ppEclbo{\pgfplotsretval}
			\pgfplotstablegetelem{0}{5}\of\Data

			\addplot
			[
				forget plot,
				mark	= none,
				color	= colorB,
				thick,
				domain	= 0:0.02,
				samples	= 100,
			]
			{quadFct(\ppEclbo,\ppEblbo,\ppEalbo)};
		\end{axis}
	\end{tikzpicture}
	\caption
	{
		\label{fig:ppdmrg:finite-size-scaling:t-\t_w-\w_g-\g:order-parameter}
		Finite size scaling for the \gls{CDW} order-parameter of the Holstein model.
		The model is evaluated for parameters $\omega/t=\protect\ReplaceStr{\w}$, $\gamma/t=\protect\ReplaceStr{\g}$ at nearly half filling where we set $N_{\rm el}=\frac{L-1}{2}$.
	}
\end{figure}

\def\Ls{51, 101, 151, 201, 251, 301, 401, 501, 601, 701, 801, 901, 1001}
\def\dw{1em10}
\def\t{1p0}
\def\w{1p0}
\def\g{1p5}
\def\blas{mkl}
\def\m{2000}
\def\nph{63}
\def\nphlbo{31}
\def\xmin{301}%
\def\xmax{51}%
\def\legendPosition{(0.03,0.03)}%
\setboolean{rebuildCurrentBlock}{false}
\setboolean{buildCurrentBlockInline}{true}

\def\Ls{51, 101, 151, 201}
\def\dw{1em10}
\def\t{1p0}
\def\w{1p0}
\def\g{2p0}
\def\blas{mkl}
\def\m{2000}
\def\nph{63}
\def\nphlbo{31}
\def\xmin{201}%
\def\xmax{51}%
\def\legendPosition{(0.03,0.75)}%
\setboolean{rebuildCurrentBlock}{false}
\setboolean{buildCurrentBlockInline}{true}
